# Supplementary material for: Learning A Single Network for Scale-Arbitrary Super-Resolution
Source: arXiv:2004.03791 source file (2021-07-23)

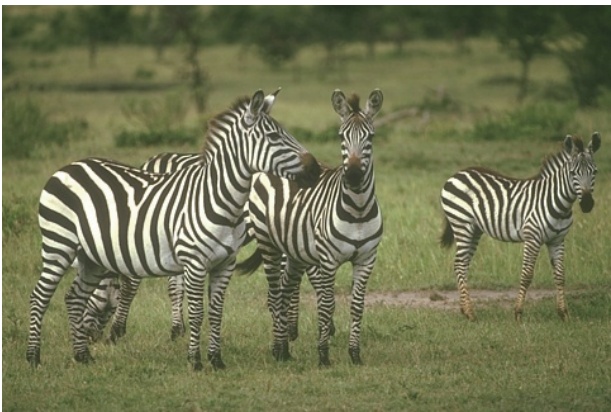

EDSR

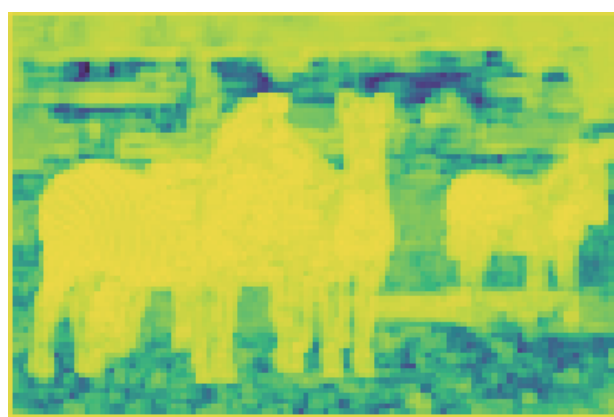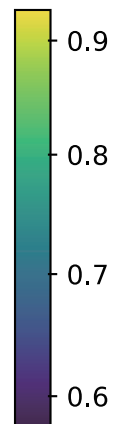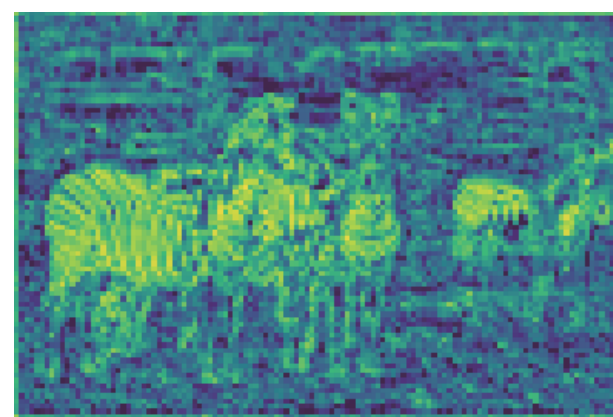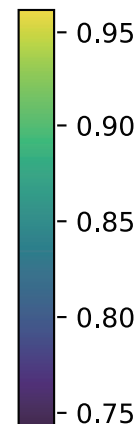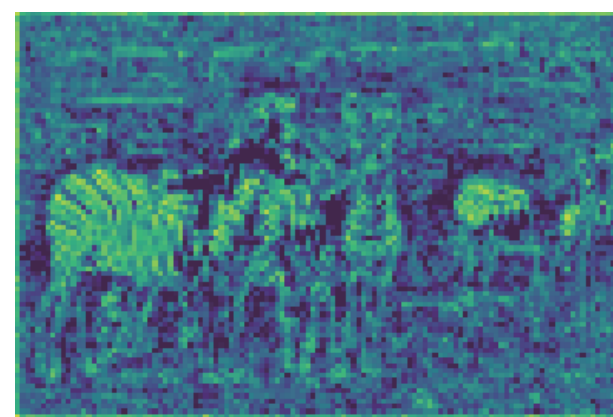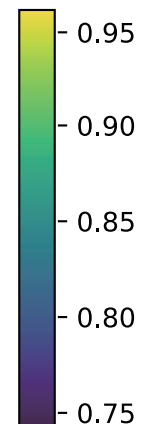

RCAN

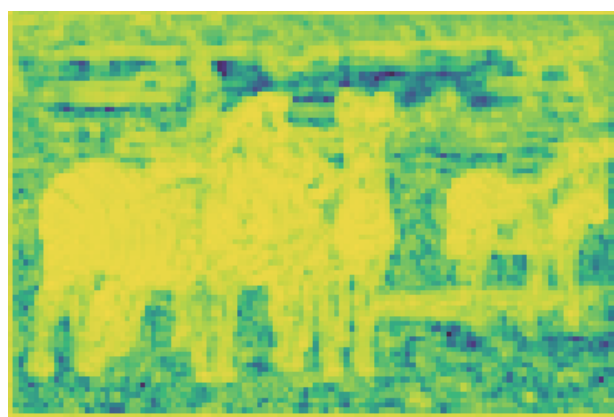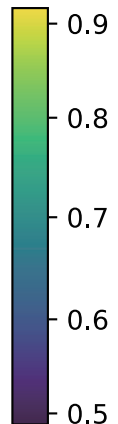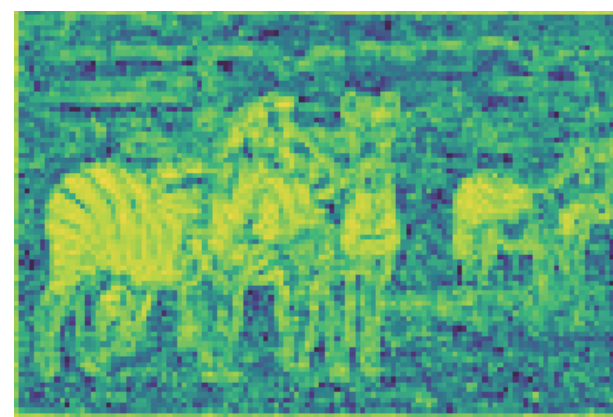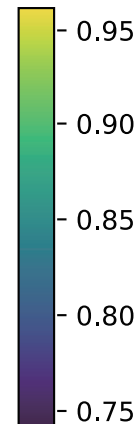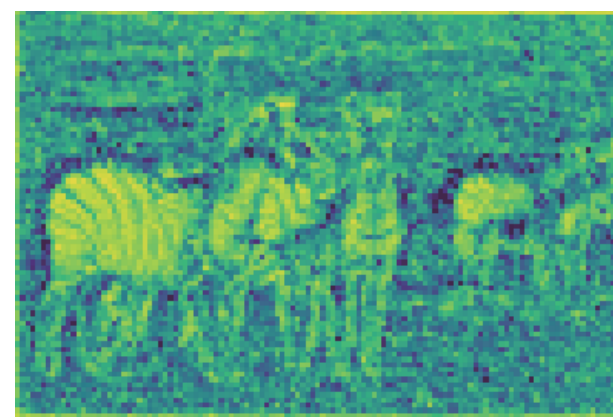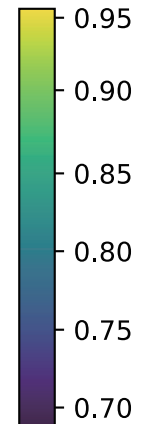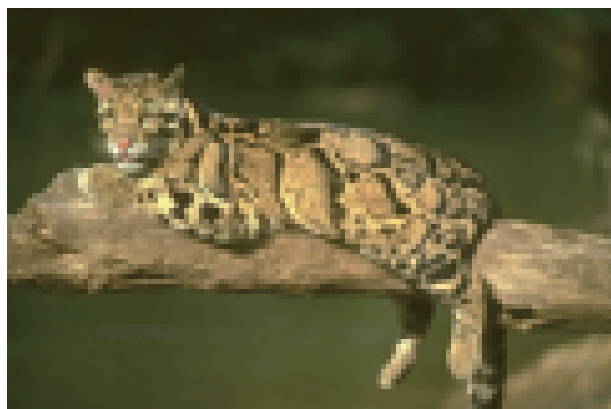

EDSR

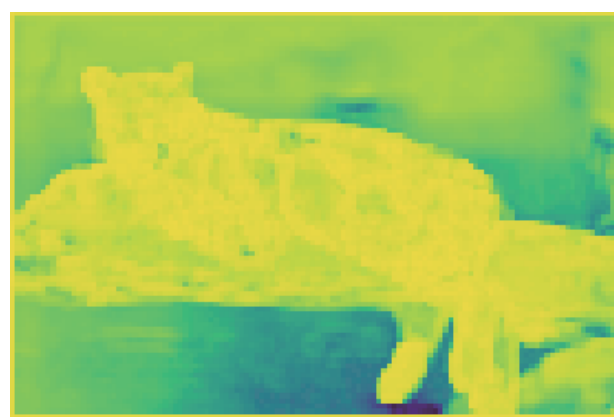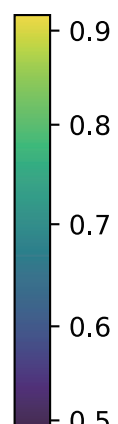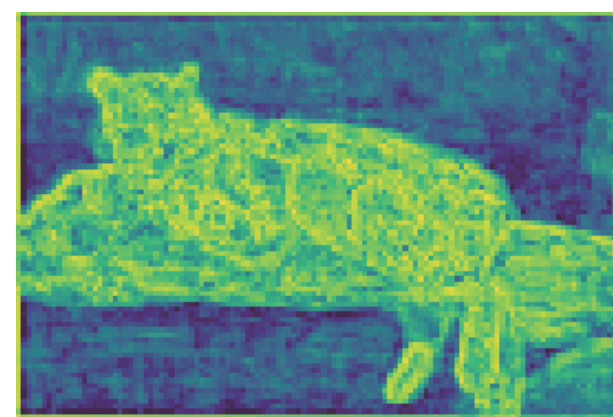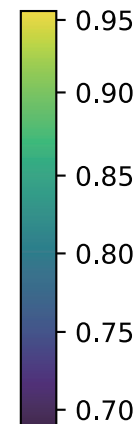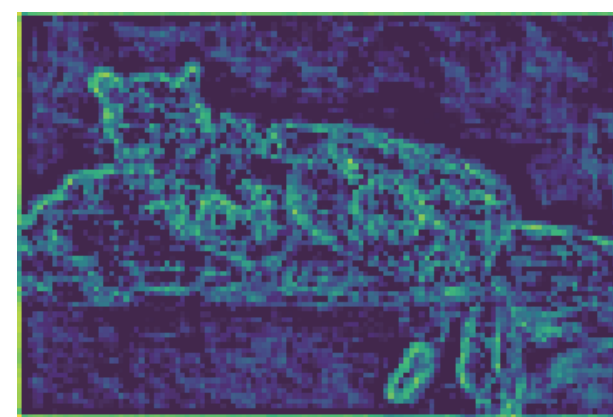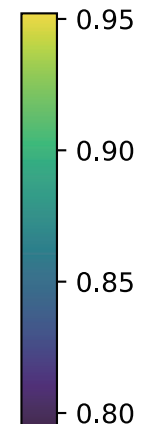

RCAN

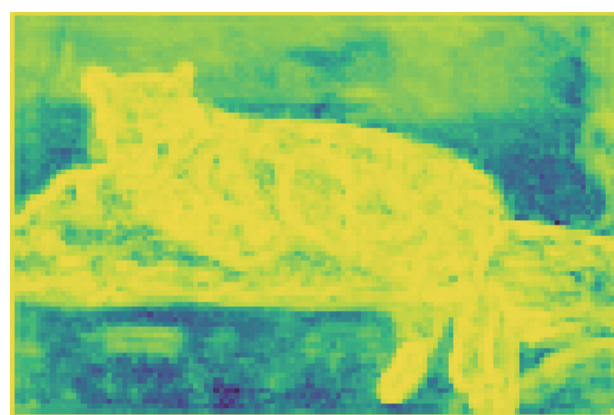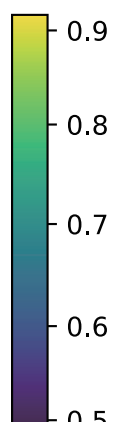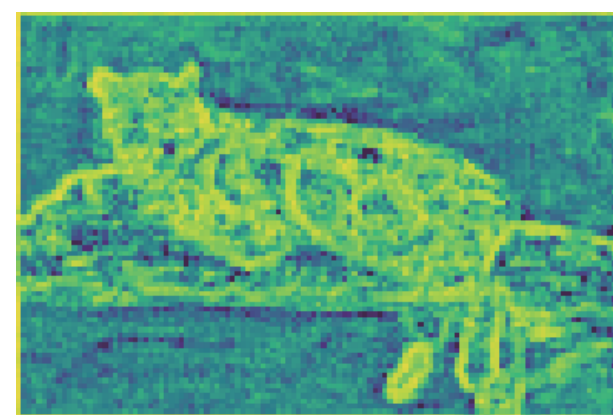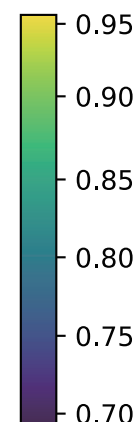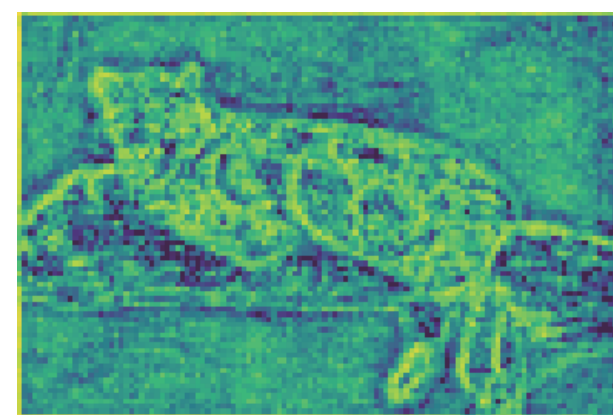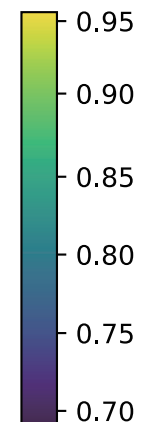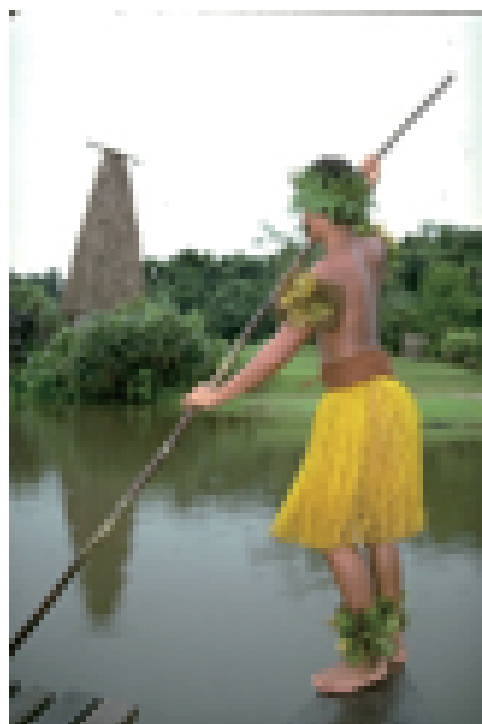

EDSR

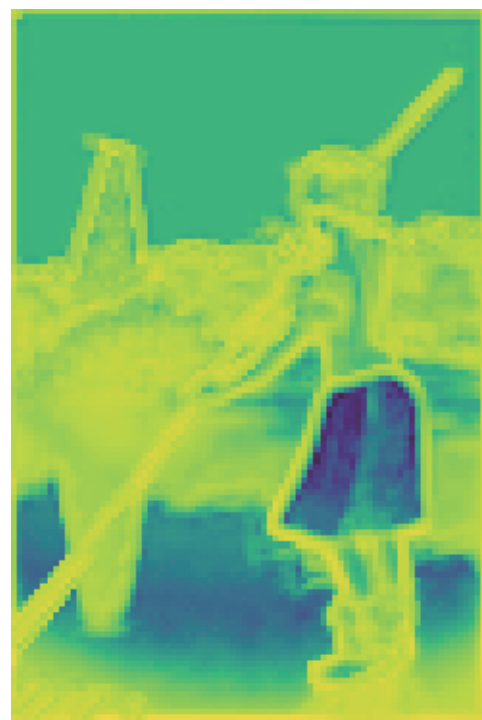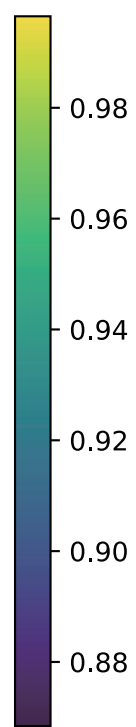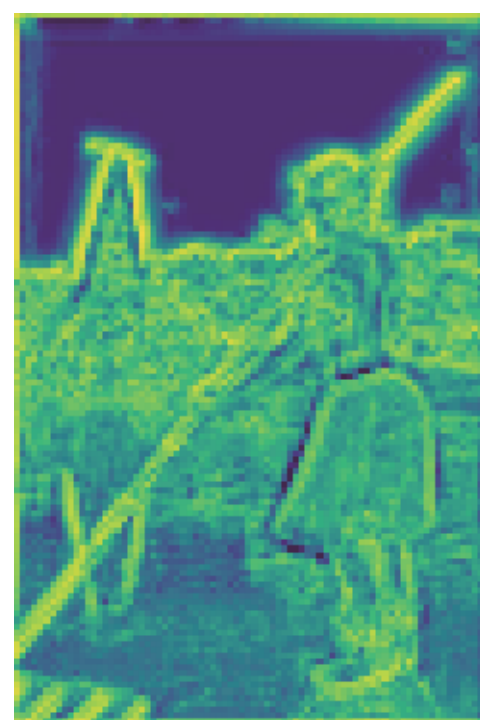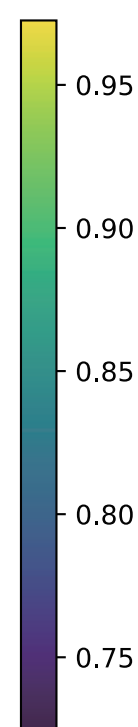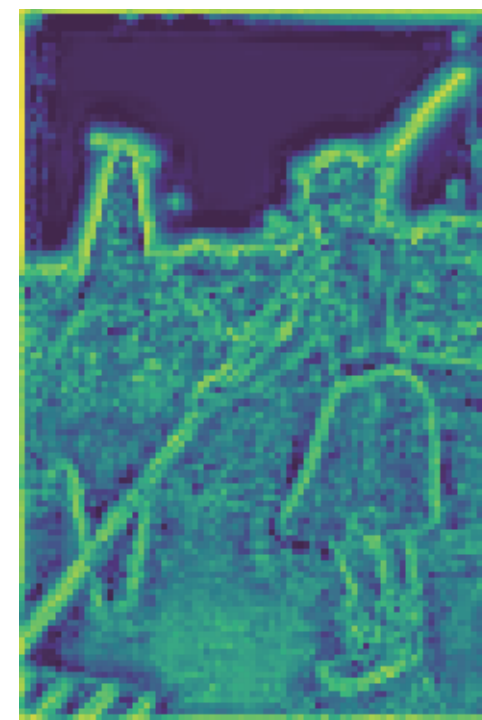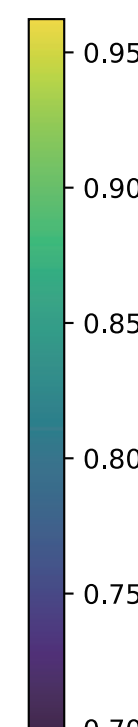

RCAN

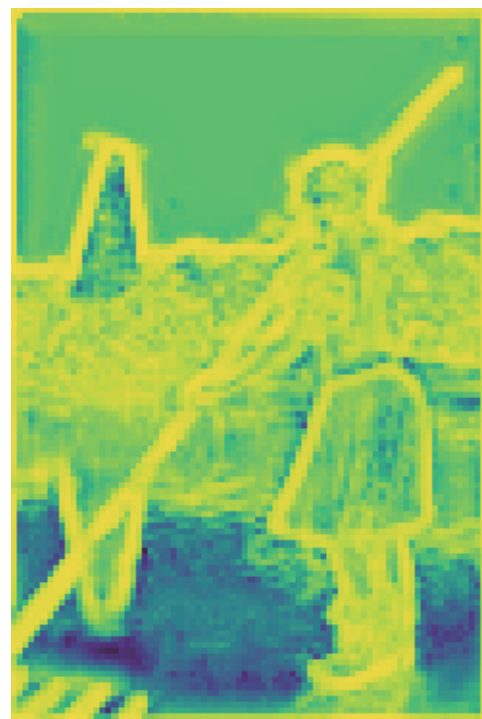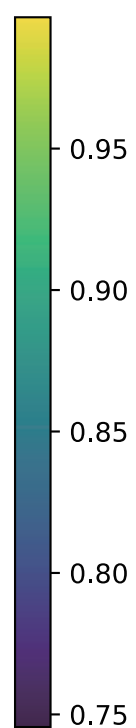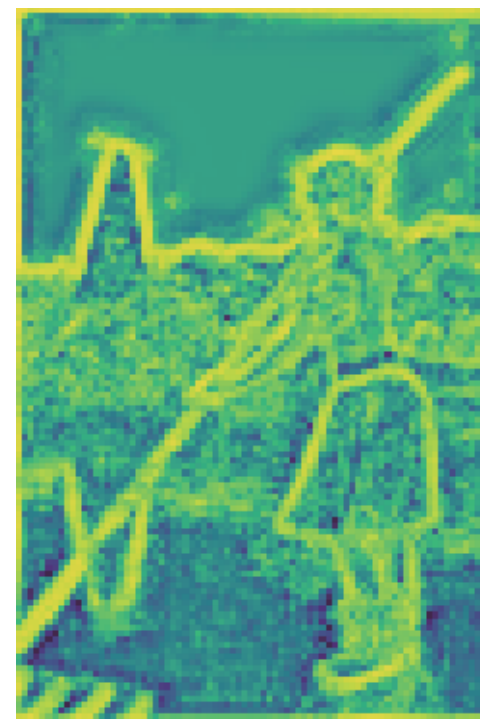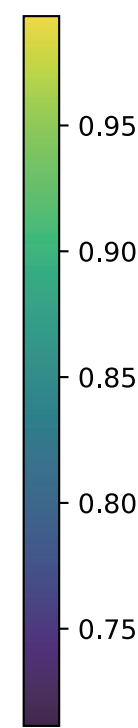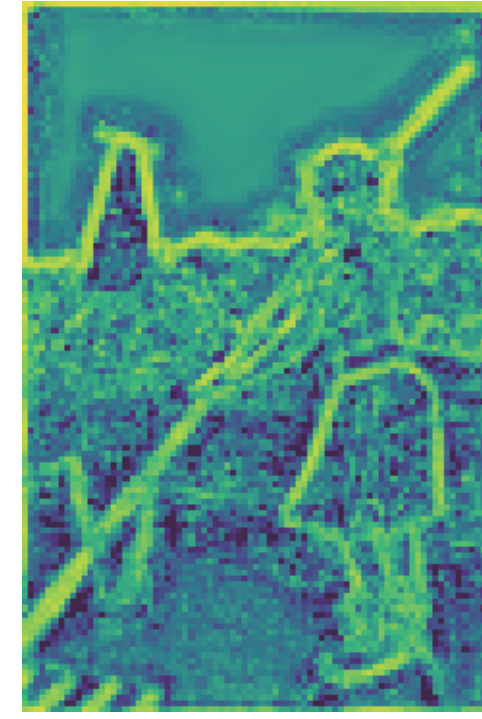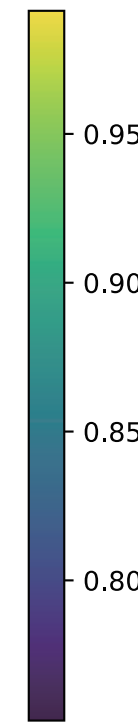

Supplement: Supplementary file 1 [file fig1_V3.pdf]
